# Supplementary material for: Unsteady aerodynamics of porous aerofoils
Source: arXiv:1911.07382 source file (2020-11-21)
Supplement: Supplementary file 1 [file appendix-endpoints.tex]

\section{Endpoint behaviour}

In this section we adapt the results of \cite[\S 29]{NIM} to obtain the asymptotic behaviour at the endpoints of the singular integral equations. 

We write

\begin{align}
    \Phi(z) = \frac{1}{2 \pi \i} \int_{-1}^1 \frac{(1-\tau)^\alpha}{(1+\tau)^\beta}\cdot \frac{\phi^\ast(\tau) }{\tau-z} \d \tau,
\end{align}

and

\begin{align}
    \Phi(t) = \frac{1}{2 \pi \i} \dashint_{-1}^1 \frac{(1-\tau)^\alpha}{(1+\tau)^\beta}\cdot \frac{\phi^\ast(\tau) }{\tau-t} \d \tau,
\end{align}
where $\phi^\ast(z)$ is an analytic function on $[-1,1]$.

\subsection{Leading edge behaviour: $t = -1$}
 The leading edge behaviour follows directly from \cite[ 29.8]{NIM}
 
 \begin{align}
     \Phi(t) =  \frac{\cot(\beta \pi)}{2 \i } \cdot \frac{(1-t)^\alpha}{(1+t)^\beta}\cdot  \phi^\ast(t) + \Phi^\ast(t)
     \label{Eq:LEAsymptotics}
 \end{align}
 
 where, in the case $\beta \neq 0$,
 
 \begin{align*}
 \Phi^\ast(t) &= \frac{\Phi^{\ast \ast}(t)}{(1+t)^{\beta_0}},
 \end{align*}
 where $\Phi^{\ast \ast}(t)$ satisfies the H\"older condition near and at $-1$ and $\beta_0<\beta$.
 
\subsection{Trailing edge behaviour: $t = 1$}

We now adapt the approach of \cite[\S 30 \& 31]{NIM} to find the second order asymptotic behaviour of $\Phi(t)$ at $t=1$. 

We may write 

\begin{align*}
    \Phi(t) &= \frac{1}{2 \pi \i} \dashint_{-1}^1 \frac{(1-\tau)^\alpha}{(1+\tau)^\beta}\cdot \frac{\phi^\ast(\tau) }{\tau-t} \d \tau \\
    & = \frac{1}{2 \pi \i} \cdot \frac{\phi^\ast (t) }{ (1+t)^\beta } \dashint_{-1}^1  \frac{(1- \tau)^\alpha}{\tau-t} \d \tau + \frac{1}{2 \pi \i} \int_{-1}^1 \left( \frac{\phi^\ast(\tau)}{(1+\tau)^\beta} - \frac{\phi^\ast(t)}{(1+t)^\beta}\right)\cdot \frac{(1 - \tau)^\alpha }{\tau-t} \d \tau \\
\end{align*}

We label the last term $\Phi_0$ and it is analytic on $[-1,1]$ and posses a Taylor expansion at the trailing-edge:

\begin{align*}
    \Phi(t) &= \frac{1}{2 \pi \i} \cdot \frac{\phi^\ast (t) }{ (1+t)^\beta } \dashint_{-1}^1  \frac{(1- \tau)^\alpha}{\tau-t} \d \tau  + \Phi_0(t).\\
\end{align*}

We note that 

\begin{align*}
    \left[ (1-z)^\alpha \right]^\pm &= \left|1-t \right|^\alpha \e^{\i \pm \alpha \pi} =(1- t)^\alpha \e^{\i (1\mp 1) \alpha \pi}.
\end{align*}

Consequently, 

\begin{align*}
\Delta \left[ (1-z)^\alpha \right]^\pm &=  (1- t)^\alpha \cdot  \left( 1 - \e^{2 \i \alpha \pi}\right) = (1- t)^\alpha \phi^\ast(t) \cdot 2 \i \e^{\i \alpha \pi} \sin(\alpha \pi), \\
\Sigma \left[ (1-z)^\alpha \right]^\pm &= (1- t)^\alpha \cdot  \left( 1 + \e^{2 \i \alpha \pi} \right) = (1- t)^\alpha \phi^\ast(t) \cdot 2 \e^{\i \alpha \pi} \cos(\alpha \pi) .
\end{align*}

Therefore, 

\begin{align*}
A(z) \coloneqq \Phi(z) - \frac{ (1-z)^\alpha }{(1 + z)^\beta} \cdot \frac{\phi^\ast(z)}{2 \i \e^{\i \alpha \pi} \sin( \alpha \pi)}
\end{align*}
defines a function that is analytic near $t=1$. Therefore, there exists a Taylor series at the trailing edge of the form

\begin{align*}
        A(t) =  A(1) + A^{\prime}(1) (t-1) + \frac{1}{2 !} A^{\prime \prime}(1) (t-1)^2\dots && \textnormal{as } t \rightarrow 1
\end{align*}

Consequently, we may write

\begin{align}
    \Sigma \left[ \Phi^\pm(z) \right]^\pm& = \frac{1}{2 \pi \i} \dashint_{-1}^1 \frac{(1-\tau)^\alpha}{(1+\tau)^\beta}\cdot \frac{\phi^\ast(\tau) }{\tau-t} \d \tau \notag\\
    &= A(1) + \Phi_0(1) - \i \frac{(1- t)^\alpha}{(1 + t)^\beta} \phi^\ast(t) \cdot \cot(\alpha \pi) + \mathcal{O}(1-t) & \textnormal{as } t \rightarrow 1 \label{Eq:TEAsymptotics}
\end{align}

\subsection{General approach} 

 We note the Plemelj formulae [cite Fokas]

\begin{align}
    \Phi^\pm(t) =  \pm \frac{(1-t)^\alpha}{(1+t)^\beta} \cdot \frac{\phi^\ast(t)}{2} + \frac{1}{2 \pi \i} \dashint_{-1}^1 \frac{(1-\tau)^\alpha}{(1+\tau)^\beta}\cdot \frac{\phi^\ast(\tau) }{\tau-t} \d \tau
\end{align}

We define

\begin{align*}
    w(z) = \frac{(1-z)^\alpha}{(1+z)^\beta} \cdot \phi^\ast(z)
\end{align*}

and note that 

\begin{align*}
    \left[ (1-z)^\alpha \right]^\pm &= \left|1-t \right|^\alpha \e^{\i \pm \alpha \pi} &&= (1- t)^\alpha \e^{\i (1\mp 1) \alpha \pi}\\
\left[ (1+z)^{-\beta} \right]^\pm& = \left|1+t \right|^{-\beta} \e^{ -\i (1\mp1) \beta \pi} &&  = (1+t )^{-\beta} \e^{ \pm \i \beta \pi} 
\end{align*}

So

\begin{align*}
\left[w(z)\right]^\pm &= \frac{ (1- t)^\alpha \e^{\i (1\mp 1) \alpha \pi}}{(1+t )^{\beta} \e^{ \mp \i \beta \pi}  } \phi^\ast(t)
\end{align*}

Consequently, 

\begin{align*}
\Delta \left[w(z)\right]^\pm &= \frac{ (1- t)^\alpha }{(1+t )^{\beta} } \phi^\ast(t) \cdot  \left( \frac{1}{\e^{-\i \beta \pi}} - \frac{\e^{2 \i \alpha \pi}}{\e^{\i \beta \pi}} \right) &= \frac{ (1- t)^\alpha }{(1+t )^{\beta} } \phi^\ast(t) \cdot 2 \i \e^{\i \alpha \pi} \sin((\beta - \alpha) \pi) \\
\Sigma \left[w(z)\right]^\pm &= \frac{ (1- t)^\alpha }{(1+t )^{\beta} } \phi^\ast(t) \cdot  \left( \frac{1}{\e^{-\i \beta \pi}} + \frac{\e^{2 \i \alpha \pi}}{\e^{\i \beta \pi}} \right) &= \frac{ (1- t)^\alpha }{(1+t )^{\beta} } \phi^\ast(t) \cdot 2 \e^{\i \alpha \pi} \cos((\beta - \alpha) \pi)
\end{align*}

Therefore, 

\begin{align*}
A(z) \coloneqq \Phi(z) - \frac{w(z) }{2 \i \e^{\i \alpha \pi} \sin((\beta - \alpha) \pi)}
\end{align*}
defines a function that is analytic along the cut $[-1,1]$. Therefore, there exist Taylor series at the leading and trailing edges of the form

\begin{align}
    A(t) = A(-1) + A^{\prime}(-1) (t+1) + \frac{1}{2 !} A^{\prime \prime}(-1) (t+1)^2\dots & \textnormal{as } t \rightarrow -1\\
        A(t) =  A(\phantom{-}1) + A^{\prime}(\phantom{-}1) (t-1) + \frac{1}{2 !} A^{\prime \prime}(\phantom{-}1) (t-1)^2\dots & \textnormal{as } t \rightarrow \phantom{-}1
\end{align}

A particular consequence of this is that 

\begin{align*}
    \Sigma \left[\Phi(z)\right]^\pm = \frac{1}{\pi \i} \dashint_{-1}^1 \frac{(1-\tau)^\alpha}{(1+\tau)^\beta}\cdot \frac{\phi^\ast(\tau) }{\tau-t} \d \tau = -\i \frac{(1-t)^\alpha}{(1+t)^\beta} \cdot \phi^\ast(t) \cot ((\beta - \alpha) \pi ) + A(\pm1)
\end{align*}

\subsection{Circulatory contributions} \label{Ap:CircTE}

We take \eqref{Eq:SVCcirc} and write the right hand side as

\begin{align*}
\frac{- \i \helmNum}{2\pi}\int_{1}^{\infty}\frac{\e^{\i \helmNum \xi}}{\xi-x} \d \xi &= -\frac{\i \helmNum}{2 \pi} \e^{\i \helmNum x} \log (1 - x) - \frac{ \i \helmNum}{2\pi}\int_{1}^{\infty}\frac{\e^{\i \helmNum \xi} - \e^{\i \helmNum x}}{\xi-x} \d \xi
\end{align*}

Consequently, we require the left hand side of \eqref{Eq:SVCcirc} to have a log singularity at $x=1$ with the correct intensity, i.e.

\begin{align*}
    \vortC(1) & = - \i \helmNum \e^{\i \helmNum}.
\end{align*}

\subsection{Limiting behaviour at discontinuities on contour}

This section is similar to \cite[\S 33]{NIM}. Consider

\begin{align*}
\Phi(z) &= \frac{1}{2 \pi \i} \int_L \frac{\phi(x)}{x-t} \d x
\end{align*}
where $\phi(t)$ has a discontinuity at $t=c$. Assume that $\phi(t)$ takes the form

\begin{align*}
\phi(t) &= \phi^\ast (t-c)^\lambda, & \gamma = \alpha + \i \beta, \qquad 0 \leq \alpha < 1
\end{align*}

where $\phi^\ast$ satisfies the H\"older condition on each of the closed contours.

Then we have, at $z \rightarrow c$,

\begin{enumerate}
	\item If $\gamma = 0$ then 
	\begin{align*}
	\Phi(z)&= \frac{\phi(c^+)-\phi(c^-)}{2 \pi \i} \log \left(\frac{1}{z - c}\right) + \Phi_0(z)
	\end{align*}
	
	\item If $\gamma = \alpha + \i \beta \neq 0$
	\begin{align*}
		\Phi(z) &= \frac{\e^{\i \gamma \pi} \phi^{\ast}(c^+) - \e^{-\i \gamma \pi} \phi^\ast(c^-)}{2 \i \sin(\gamma \pi)} \cdot \left(z - c\right)^\gamma + \Phi_0(z)
	\end{align*}
\end{enumerate}

If $z = t_0 \rightarrow c$ then

\begin{enumerate}
	\item If $\gamma = 0$ then 
	\begin{align*}
	\Phi(z)&= \frac{\phi(c^+)-\phi(c^-)}{2 \pi \i} \log \left(\frac{1}{t_0 - c}\right) + \Phi_0^\ast(t_0)
	\end{align*}
	
	\item If $\gamma = \alpha + \i \beta \neq 0$
	\begin{align}
	\Phi(z) &= \begin{dcases}
\left(-\frac{\e^{-\i \gamma \pi} }{2 \i \sin(\gamma \pi)} \phi^{\ast}(c^+) + \frac{\cot(\gamma \pi)}{2 \i } \phi^\ast(c^-) \right) \cdot \left(t_0 - c\right)^\gamma + \Phi_0^\ast(t_0) & t_0 \rightarrow c^-\\
\left(\phantom{-} \frac{\e^{\i \gamma \pi}}{2 \i \sin(\gamma \pi)} \phi^{\ast}(c^-) - \frac{\cot(\gamma \pi)}{2 \i } \phi^\ast(c^+) \right) \cdot \left(t_0 - c\right)^\gamma + \Phi_0^\ast(t_0) & t_0 \rightarrow c^+ 
\end{dcases}
	\label{Eq:plemeljDiscLim}
	\end{align}
\end{enumerate}

A "validation" of the last result is available in \texttt{plemelj-limit-checks.nb}.
