# Supplementary material for: Unsteady aerodynamics of porous aerofoils
Source: arXiv:1911.07382 source file (2020-11-21)
Supplement: Supplementary file 2 [file appendix-uniqueness.tex]

\section{Uniqueness of singular Fredholm--Volterra operator}

In this appendix we prove that the solutions subjects to a specified singular or non-singular behaviour at the endpoints.

We consider two solutions that possess the same singular behaviour at the endpoints, $\gamma_1$ and $\gamma_2$. We define $\gamma_\Delta = \gamma_1 - \gamma_2$. The solutions $\gamma_{1,2}$ each satisfy a H\"older condition, so there exist non-negative, real constants $\alpha_{1,2}>0$ and $C_{1,2}$ such that
\begin{align*}
\left| \gamma_n(x) - \gamma_n(y)\right| \leq C_n \left| x - y\right|^{\alpha_n}, \qquad \textnormal{for } n  = 1,2,\\
\end{align*}
for all $-1<x,y<1$. Consequently, we may write
\begin{align}
\left| \gamma_\Delta(x) - \gamma_\Delta(y) \right| \leq C_1 \left| x-y\right|^{\alpha_1} \left(1+ \frac{C_2}{C_1} \left| x-y\right|^{\alpha_2-\alpha_1} \right).  \label{Eq:holProof}
\end{align}
We may assume (without loss of generality) that $\alpha_2>\alpha_1$. Since $x$ and $y$ are bounded, the final bracketed term in \eqref{Eq:holProof} is therefore also bounded. Consequently, $\gamma_\Delta$ also satisfies a H\"older condition.

We now $\mathcal{L}[\gamma_\Delta]\equiv 0 $ to obtain the expression
\begin{align}
 \psi(x) \gamma_\Delta(x)- \frac{1}{\pi}\dashint_{-1}^{1}\frac{\gamma_\Delta(\xi)}{\xi-x}\d \xi&= - \i \helmNum \psi(x) \int_{-1}^x \gamma_\Delta(\xi) \d \xi. \label{Eq:SIE1}
\end{align}
We may also use the expression
\begin{align*}
\dashint_{-1}^{1}\frac{\gamma_\Delta(\xi)}{\xi-x}\d \xi = \gamma_\Delta(x)\log\left(\frac{1-x}{1+x}\right) + \dashint_{-1}^{1} \frac{\left(\gamma_\Delta(\xi)-\gamma_\Delta(x)\right)}{\xi-x}\d \xi
\end{align*}
to rewrite \eqref{Eq:SIE1} as 
\begin{align*}
\gamma_\Delta(x) & = \frac{\pi}{\log\left((1-x)/(1+x)\right)} \left(  \psi(x) \gamma_\Delta(x)- \frac{1}{\pi}\dashint_{-1}^{1}\frac{\left(\gamma_\Delta(\xi)- \gamma_\Delta(x) \right)}{\xi-x}\d \xi+ \i \helmNum \psi(x) \int_{-1}^x \gamma_\Delta(\xi) \d \xi  \right) 
\end{align*}
Try Poincare--Bertand?

In the case that $\gamma_\Delta$ is bounded at one end and unbounded at the other, \eqref{Eq:uniSIE} may be rearranged in the unique form
\begin{align*}
\gamma_\Delta(x) &= -\i\frac{\helmNum (\psi(x))^2}{1+(\psi(x))^2} \int_{-1}^x \gamma_\Delta(\xi) \d \xi + \\
& + \frac{Z(x)}{1 + (\psi(x))^2} \dashint_{-1}^1 \left( - \i \helmNum \psi(\xi) \int_{-1}^\xi \gamma_\Delta(\tau) \d \tau \right) \frac{ \d \xi}{Z(\xi) ( \xi - x)}
\end{align*}
We now use the inequalities
\begin{align*}
\left|\int_{-1}^x \gamma_\Delta(\xi) \d \xi \right|  \leq \left| x \right| \left\|\gamma_\Delta(\xi) \right\|_\infty
\end{align*}
